# Supplementary material for: RoboAssembly: Learning Generalizable Furniture Assembly Policy in a Novel Multi-robot Contact-rich Simulation Environment
Source: arXiv:2112.10143 source file (2021-12-19)
Supplement: Supplementary file 1 [file supp.tex]

\subsection{Notation Table}
We create a notation table shown in Table~\ref{tab:notation} summarizing the symbols used in this work.
\begin{table}[hbt!]
\begin{tabular}{@{}p{0.15\linewidth}|p{0.75\linewidth}}  
\hline \hline
Symbol & explanation\\
\hline
$s$ & the state in the RL setting\\
$a$ & the action in the RL setting\\
$r$ & the reward in the RL setting \\
$N_{train}$ & the total number of chairs in the training set\\
$N_{test}$ & the total number of chairs in the test set\\
$\mathcal{Z}^i$ & the chair with an id of $i$\\
$M_i$ & the total number of parts in the chair $\mathcal{Z}^i$\\
$\mathcal{P}^i_x$ & the part with an id of $x$ in the chair\\
$\mathcal{J}^{i}_{x,y}$ & the joint with an id of $y$ in the part $\mathcal{P}^i_x$\\
$K^i_x$ & the total number of joints of the part $\mathcal{P}^i_x$\\
$\mathcal{C}^i$ & the joint connection status tensor of the chair $\mathcal{Z}^i$\\
$\mathcal{T}^i_{t,x}$ & the absolute 6D pose of the part $\mathcal{P}^i_x$ at the time step $t$\\
$\mathcal{T}^i_{t,(u,v)}$ & the relative 6D pose transformation between part $\mathcal{P}^i_u$ and part $\mathcal{P}^i_v$ at the time step $t$\\
$^\mathcal{J}\mathcal{T}^{i}_{x,y}$ & the local transformation of the joint connection $\mathcal{J}^i_{x,y}$ on the part\\
$^\mathcal{G}\mathcal{T}^{i}_{x}$ & the grasable region annotated on the part $\mathcal{P}^i_x$\\
$X^i_{0,x}$ & the sampled point cloud of the part $\mathcal{P}^i_x$ at the initial time step $t=0$\\
$m$ & the number of point in the $X^i_{0,x}$\\
% 两个 robot 对应的 symbol
\hline\hline
\end{tabular}\caption{Notation Table}\label{tab:notation}
\end{table}

\subsection{Step fuction}\label{sec:step}
\begin{algorithm}[h!]  
  \caption{Step Function: 
  Input(general: $u$, $v$, $k$, $l$; 
  w/o robot: $\text{pose connect id}$; 
  with robot: $a$, $b$)}  
  \label{alg:w/o & with robot}  
  \begin{algorithmic}[1]  
    \State Initialize parts on the ground (w/o robot) or on corresponding holder (with robot), and two robots R$_1$  R$_2$ (with robot)
    \While{not done}
        \State Prep\_success\_flag = False
        \State Merge\_success\_flag = False
        % deal with equivalent part
        \State Gather all parts which are geometrically equivalent to $\mathcal P_u^i$, denoted as $Set(\mathcal{P}_u^i)$  \mingxin{Here these parts have the same joint}
        \State $\mathcal{P}_{u'}^i$. Find the part $\mathcal P_{u'}^i$ connects to $\mathcal P_v^i$ with $\mathcal J^i_{v,l}$ and the part $\mathcal P_{v'}^i$ connects to $\mathcal P_{u'}^i$ with $\mathcal J^i_{u,k}$.
        
        \If {$\mathcal P_{u'}^i \in G$ and $\mathcal P_{v'}^i==\mathcal P_{v}^i$} {}
            \If {w/o robot setting}{}
                \State adjust pose of $\mathcal P_{v}^i$ group based on $a_{\text{quat}, c}$ 
                \State Prep\_success\_flag $\gets$ True
            \ElsIf{with robot setting}
                \State Plan a path for R$_1$ to grasp $\mathcal P_u^i$
                \State Plan a path for R$_2$ to grasp $\mathcal P_v^i$
                \If {both paths are found within time limit}{}
                    \State Prep\_success\_flag $\gets$ True
                    \State R$_1$ and R$_2$ execute the paths in turn
                    \State Move R$_2$ towards default xy pose \lin{Explain what is default xy pose} % 只是朝对应方向走若干步，并非完全 reset to default xy pose
                \EndIf
            \EndIf
            \If{Prep\_success\_flag == True}{}
                \State Plan a path to move $\mathcal{P}^i_u$ \mingxin{w/o robot: self-driven; with robot: held by R$_1$} to the calculated pose of $\mathcal{P}^i_{u'}$
                \If {path is found within time limit}{}
                    \State execute planned path
                    \State merge the two group as one
                    \If{w/o robot setting}{}
                        \State Merge\_success\_flag $\gets$ True
                    \ElsIf{with robot setting}
                        \State R$_1$ free the gripper
                        \State Plan a path for R$_2$ to position held group on corresponding holder
                        \If {path is found within time limit}{}
                            \State R$_2$ execute path and free gripper
                            \State R$_1$ \& R$_2$ reset to default pose
                            \State Merge\_success\_flag $\gets$ True
                        \EndIf
                    \EndIf
                \EndIf
            \EndIf
        \EndIf
        \If {Merge\_success\_flag == True}{}
            \If {the chair has been assembled successfully}{}
                \State $\mathcal R \gets 5 $
                \State $done$ $\gets$ True
            \Else
                \State $\mathcal R \gets 1 $
                \State $done$ $\gets$ False 
            \EndIf
        \Else
            \State $\mathcal R \gets 0$
            \State $done$ $\gets$ True
        \EndIf
        \State Update 6D-pose, joint matrix in state
    \EndWhile
  \end{algorithmic}  
\end{algorithm}\label{alg:step}
